# Supplementary material for: Experimental Performance of Blind Position Estimation Using Deep Learning
Source: arXiv:2306.03721 source file (2023-06-06)
Supplement: Supplementary file 1 [file 08_appendix.tex]

\appendix[Derivation of ]
